# Supplementary material for: Systematic partitioning of proteins for quantum-chemical fragmentation methods using graph algorithms
Source: arXiv:2010.02832 ancillary file (2020-12-18)
Supplement: Supplementary file 1 [file si.pdf]

# Systematic partitioning of proteins for quantum-chemical fragmentation methods using graph algorithms

Mario Wolter[a], Moritz von Looz[b,c], Henning Meyerhenke[b,1], and Christoph R. Jacob [a,2]

[a] Technische Universität Braunschweig, Institute of Physical and Theoretical Chemistry, Gaußstraße 17, 38106 Braunschweig, Germany

[b] Department of Computer Science, Humboldt-Universität zu Berlin, Unter den Linden 6, 10099 Berlin, Germany

[c] Now at Advanced Concepts Team, European Space Research and Technology Center, Noordwijk, The Netherlands

# Supporting Information

[1]E-Mail: meyerhenke@hu-berlin.de

[2]E-Mail: c.jacob@tu-braunschweig.de

# S1 Comparison to supermolecular results: Sem5 SH3 domain monomer

As a second test case for assessing the two-body approximations $\Delta E^{(2)}$ and $\Delta_{\text{abs}}^{(2)}$ to the error in the Coulomb interaction energy $\Delta E$ and the absolute error $\Delta_{\text{abs}}^{(2)}$, respectively, we consider the Sem5 SH3 domain monomer (see Section 4). Here, the error measures $\Delta E$ and $\Delta_{\text{abs}}^{(2)}$ have been evaluated using a supermolecular DFT calculation for the full protein, as described for ubiquitin in Section 3.1. Fig. S1 plots the different fragmentation error measures for naïve partitions with an increasing number $n_{\text{max}}$ of amino acids per fragment (cf. the corresponding plot for ubiquitin in Fig. 4).

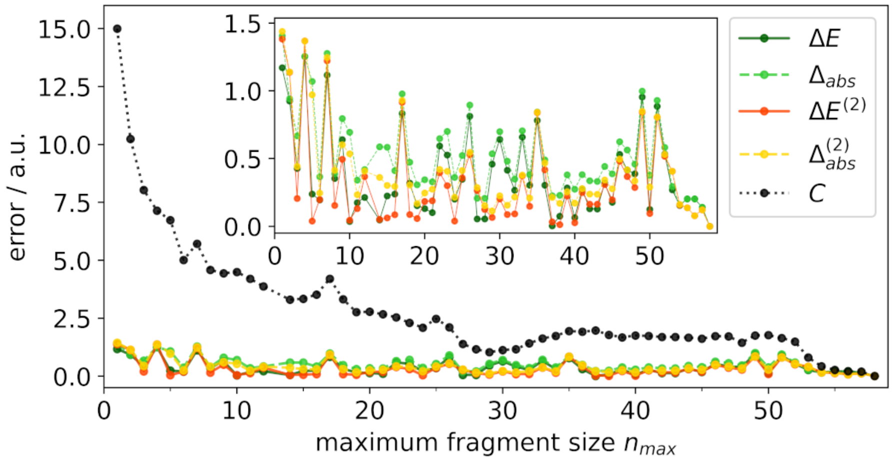


Figure S1: Comparison of fragmentation error measures $\Delta E$ (solid dark green line), $\Delta_{\text{abs}}$ (dashed green line) and error estimates $\Delta E^{(2)}$ (solid red line), $\Delta_{\text{abs}}^{(2)}$ (dashed yellow line), $C$ (dotted black line) for the Sem5 SH3 test case using naïve partitions with different maximum number of amino acids per fragment $n_{\text{max}}$. The inset shows the same data but excludes $C$.

Overall, the figure shows an excellent agreement between the two error measures $\Delta E$ and $\Delta_{\text{abs}}$ (solid dark green line and dashed light green line) and the corresponding two-body approximations $\Delta E^{(2)}$ and $\Delta_{\text{abs}}^{(2)}$ (solid red and dashed yellow line).

Fig. S2 plots the absolute error $\Delta_{\text{abs}}$ and the two-body approximation to the absolute error

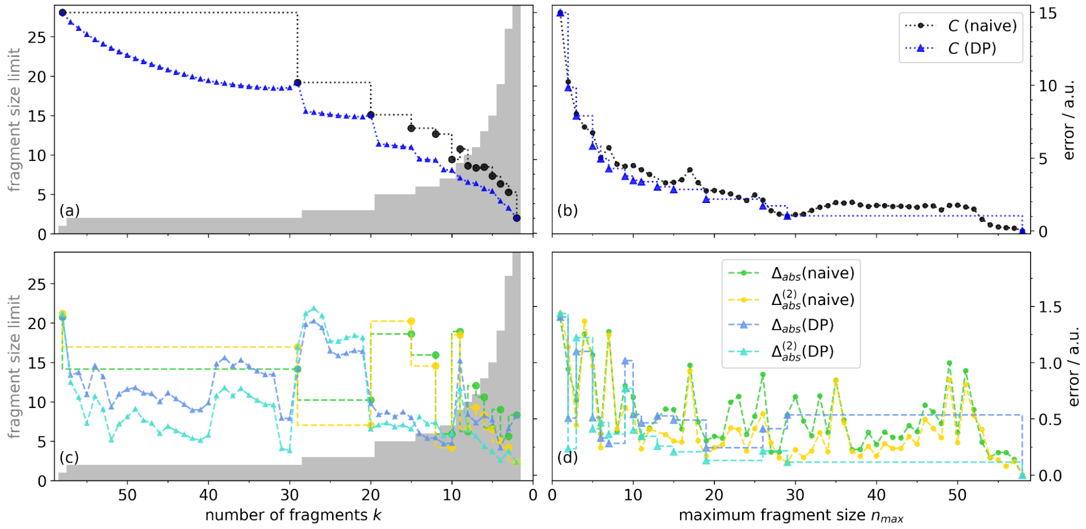


Figure S2: Comparison of the partitions obtained by the DP algorithm (triangles) and the corresponding naïve partitions (circles) for the Sem5 SH3 monomer. (a,b) Comparison of the edge cut weight. (c,d) Comparison of the absolute error $\Delta_{\text{abs}}$ (green circles and blue triangles) and the corresponding error estimate $\Delta_{\text{abs}}^{(2)}$ (yellow circles and cyan triangles). In (a) and (c) the horizontal axis shows the number of fragments $k$. The corresponding fragment size limit $n_{\max}$ applicable in the DP algorithm is shown as gray bars. In (b) and (d), the horizontal axis shows the maximum number of amino acids per fragment $n_{\max}$.

$\Delta_{\mathrm{abs}}^{(2)}$ for both the naïve partitions and the partitions obtained from the DP algorithm for the Sem5 SH3 test case (cf. the corresponding plot for ubiquitin in Fig. 5). While for the partitions of the DP algorithm, there are some differences between $\Delta_{\mathrm{abs}}$ (dashed blue lines in Fig. S2c and d) and $\Delta_{\mathrm{abs}}^{(2)}$ (dashed cyan line in in Fig. S2c and d), the overall agreement is very good and comparable to the one found for ubiquitin.

## S2 No cut-off for edge weights: Ubiquitin

In all calculations presented in the main paper, we applied a distance cut-off of 2.5 Åbetween pairs of amino acids through space in the construction of the graph representation and in the underlying two-body approximation (see Section 2.6). To assess the impact of this approximation, Fig. S3 presents the results of Fig. 4 when including all pairs of amino acids.

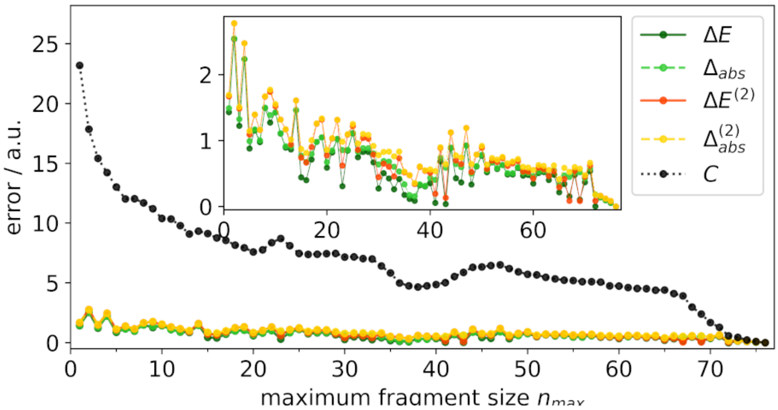


Figure S3: Comparison of fragmentation error measures $\Delta E$ (solid dark green line), $\Delta_{\mathrm{abs}}$ (dashed green line) and error estimates $\Delta E^{(2)}$ (solid red line), $\Delta_{\mathrm{abs}}^{(2)}$ (dashed yellow line), $C$ (dotted black line) for the ubiquitin test case without cut-off for calculated edge weights using naïve partitions with different maximum number of amino acids per fragment $n_{\mathrm{max}}$. The inset shows the same data but excludes $C$.

The comparison of Fig. 4 and Fig. S3 shows no obvious changes. Overall, the small

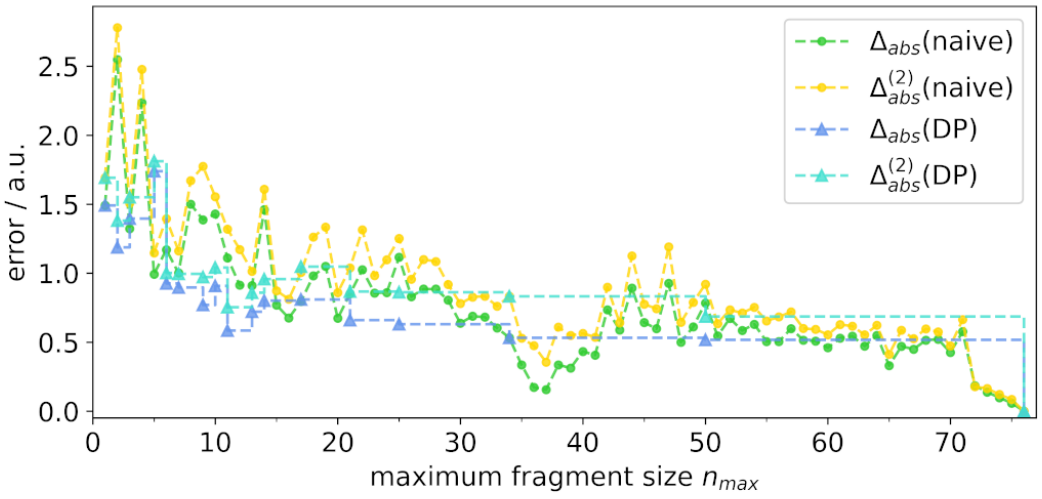


Figure S4: Comparison of the partitions obtained by the DP algorithm (triangles) and the corresponding naïve partitions (circles) for ubiquitin without cut-offs for calculated edge weights. Comparison of the absolute error $\Delta_{\text{abs}}$ (green circles and blue triangles) and the corresponding error estimate $\Delta^{(2)}_{\text{abs}}$ (yellow circles and cyan triangles). The horizontal axis shows the maximum number of amino acids per fragment $n_{\text{max}}$. See text for details.

differences between the error measures $\Delta E$ and $\Delta_{\text{abs}}$ and the corresponding two-body approximations $\Delta E^{(2)}$ and $\Delta^{(2)}_{\text{abs}}$ are slightly decreased.

When employing the complete graphs constructed without a distance cut-off, the DP algorithm results in slightly different partitions for some maximum fragment sizes. Fig. S4 presents the results corresponding to those of Fig. 5d. Overall, the similar reductions of the absolute error compared to the naïve partitions are found, even though there are differences for some fragment sizes, particularly for large $n_{\text{max}}$.
